# Supplementary material for: Few-shot Implicit Function Generation via Equivariance
Source: arXiv:2501.01601 source file (2025-01-03)
Supplement: Supplementary file 1 [file X_suppl.tex]

\clearpage
\setcounter{page}{1}
\setlength{\abovedisplayskip}{5pt} 
\setlength{\belowdisplayskip}{5pt}
\maketitlesupplementary

\section{Detailed Problem Formalization} \label{app:problem}
% For any class $f \in \mathcal{F}$, we define its weight distribution as:
% \begin{equation}
%     p_f(w) := P(w | d(\Phi(w), f) \leq \epsilon),
% \end{equation}
% where $d(\Phi(w), f) = \mathbb{E}_{x \sim \mathcal{X}} [ |\Phi(w)(x) - y_f(x)|_2^2 ]^{1/2}$ measures reconstruction quality, $y_f(x)$ represents target values for class $f$, and $\epsilon$ controls acceptable variation.

% Given training classes $\{f_1, ..., f_N\}$ with support sets $S_{f_i} = \{w_1^i,...,w_k^i\} \stackrel{i.i.d.}{\sim} p_{f_i}(w)$, we optimize:
% \begin{equation}
%     \min_\theta \mathbb{E}_{f \sim \mathcal{F}} [\mathcal{D}(G(S_f), p_f(w)) | S_f \stackrel{i.i.d.}{\sim} p_f(w)],
% \end{equation}
% where $\mathcal{D}$ measures distribution distance.

% \subsection{Problem Definition} \label{sec:def}
Following the definition we gave in the \textit{Preliminary}, we now formulate a more theoretical and official definition.

We aim to generate diverse neural network weights that encode different instances within the same signal class (\textit{e.g.}, different styles of digit "7", different shapes of planes) as implicit neural representations, given only a few example weights as reference.

Let $\mathcal{W} \subseteq \mathbb{R}^d$ denote the weight space of MLPs with a fixed architecture, where $d$ is the total number of parameters when all weights are flattened into a single vector. Consider a class space $\mathcal{F}$ where each $f \in \mathcal{F}$ represents a class of signals (\textit{e.g.}, a specific digit, a category of shapes). Let $\Phi: \mathcal{W} \rightarrow (\mathcal{X} \rightarrow \mathcal{Y})$ map weights to their corresponding implicit functions, where $\mathcal{X}$ is the coordinate space (e.g., 2D/3D coordinates) and $\mathcal{Y}$ is the target space (e.g., RGB values, occupancy).

\begin{definition}[Class-Induced Weight Distribution]
For any class $f \in \mathcal{F}$ with corresponding coordinate space $\mathcal{X}$, we define its corresponding weight distribution as:
\begin{equation}
    % p_f(w) := P(w | w \text{ encodes a valid instance of class } f),
    p_f(w) := P(w | d(\Phi(w), f) \leq \epsilon)
\end{equation}
where validity is measured by a distance metric:
\begin{equation}
    d(\Phi(w), f) = \mathbb{E}_{x \sim \mathcal{X}} \left[ |\Phi(w)(x) - y_f(x)|_2^2 \right]^{1/2},
\end{equation}
where $y_f(x)$ represents the target values for class $f$ at coordinate $x$, and $\epsilon > 0$ is a tolerance parameter that determines the acceptable variation within the class.
\end{definition}

\begin{definition}[Few-shot Weight Generation]
Given:
\begin{itemize}
    \item A set of training classes $\{f_1, ..., f_N\} \subset \mathcal{F}$ (e.g., different digits, different shape categories) with their corresponding weight distributions $\{p_{f_1}(w), ..., p_{f_N}(w)\}$
    \item For each class $f_i$, a support set $S_{f_i} = \{w_1^i,...,w_k^i\}$ where $w_j^i \stackrel{i.i.d.}{\sim} p_{f_i}(w)$ represents different MLP weights that encode valid instances of that class
\end{itemize}

The Few-shot Class-based INR Weight Generation problem is to learn a generator $G$ that can estimate the weight distribution of any class $f \in \mathcal{F}$ given only its k-shot support set:
\begin{equation}
    G: S_f \mapsto \tilde{p}_f(w),
\end{equation}
such that the generated distribution $\tilde{p}_f(w) \approx p_f(w)$ when $S_f = \{w_1,...,w_k\} \stackrel{i.i.d.}{\sim} p_f(w)$. The final objective is to minimize the expected distribution distance over the space of possible test classes:
\begin{equation}
    \min_\theta \mathbb{E}_{f \sim \mathcal{F}} [\mathcal{D}(G(S_f), p_f(w)) | S_f \stackrel{i.i.d.}{\sim} p_f(w)].
\end{equation}
\end{definition}

\section{Additional Related Work}

\subsection{Implicit Neural Representation}
Implicit Neural Representations (INRs) have demonstrated remarkable efficacy in representing diverse forms of complex signals, including spatial occupancy~\cite{occ1,wire,siren}, 3D geometric morphology~\cite{chen2019learning,chabra2020deep,genova2019learning}, signed distance functions~\cite{deepsdf,dist}, 3D scene appearence~\cite{xie2022neural,chen2023neurbf,muller2022instant,ma2023deformable,li2023dynibar} and some other complex signals~\cite{mcginnis2023single,xu2023nesvor,ma2024continuous,inr3} with the help of a small neural network, usually a MLP with few layers. 

Within this domain, several methodological innovations have emerged as particularly noteworthy. The SIREN architecture employs sinusoidal activation functions to capture high-frequency spatial details with unprecedented fidelity~\cite{siren}. Subsequent research has introduced Gaussian activation functions, offering enhanced initialization stability and parameter efficiency compared to their predecessors~\cite{inr2}. The WIRE framework represents a significant advancement through its implementation of continuous complex Gabor wavelets, enabling robust and high-precision representation of natural images~\cite{wire}. Furthermore, LIIF has introduced novel approaches to continuous representation, specifically addressing the challenge of arbitrary resolution representation~\cite{inr3}.

\subsection{Generative Models}
For image generation task, diffusion probabilistic models have revolutionized generative modeling~\cite{ddim,dhariwal2021diffusion,ddpm}, emerging as a powerful alternative to traditional approaches like GANs~\cite{gan} and energy-based models (EBMs)~\cite{ebm}. Their success in image synthesis stems from their ability to produce higher quality outputs with improved fidelity~\cite{ddim,ldm}, while also enabling effective text conditioning~\cite{glide,saharia2022photorealistic}. A notable advancement came with Latent Diffusion, which achieved efficient high-resolution image synthesis by applying the diffusion process in the latent space of pretrained autoencoders~\cite{blattmann2022retrieval,ldm}.

The extension of diffusion models to 3D domains has followed several paths. Early attempts to directly apply 2D generation techniques to 3D voxel grids encountered computational limitations at higher resolutions due to the inherent complexity of 3D convolution networks~\cite{wu2016learning,smith2017improved,lunz2020inverse}. This led researchers to explore alternative 3D representations, including point clouds~\cite{pvd,yang2019pointflow} and implicit fields~\cite{chen2019learning,mescheder2019occupancy}. A significant breakthrough came with MeshDiffusion~\cite{liu2023meshdiffusion}, which pioneered the unconditional generation of 3D shapes using diffusion models with direct 3D shape supervision.

Recent work has expanded diffusion models beyond traditional data types to address the challenge of generating neural network parameters. HyperNetworks\cite{hypernetworks} introduced the concept of using one network to learn the parameters of another. Model-Agnostic Meta-Learning (MAML) developed methods for learning parameter initializations that enable efficient fine-tuning~\cite{maml}. The G.pt model proposed predicting parameter update distributions based on initial parameters and prompted losses~\cite{Peebles2022}. Other approaches have included using autoencoders trained on model zoos to learn hyper-representations for parameter generation~\cite{wang2024neural,schurholt2022hyper}, GNN-based parameter sampling~\cite{knyazev2021parameter}, and direct MLP weight generation for neural implicit fields~\cite{hyperdiffusion}.

Most recently, diffusion models have been successfully applied to generate high-performing neural network parameters across various architectures and datasets, demonstrating their potential for weight generation tasks.

\begin{figure}[t]
    \centering
    \includegraphics[width=1\linewidth]{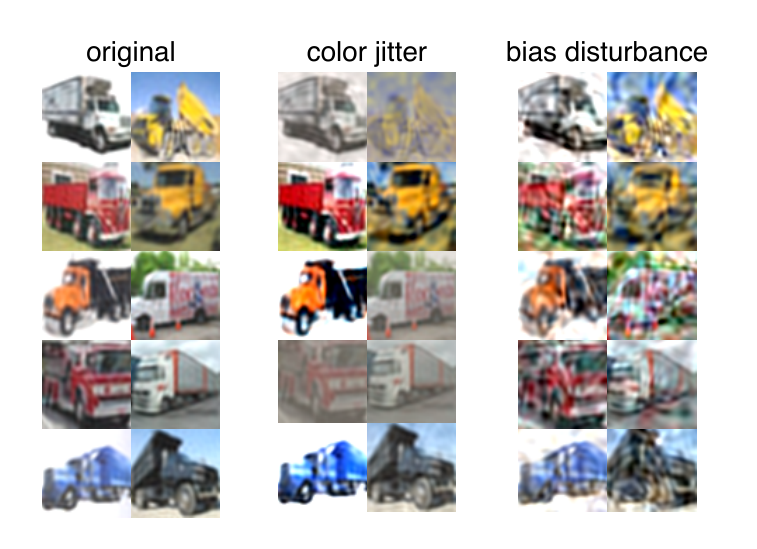}
    \caption{Visualization of the proposed INR-based data augmentation including color jitter (middle) and bias disturbance (right).}
    \label{fig:aug}
\end{figure}

\section{INR-based Data Augmentation}

% \subsection{INR-based Data Augmentation Framework}

For the INR-based data augmentation part. In our framework, we incorporate several established augmentation methods for INRs. Consider an INR that maps an image, defined as $f : \mathbb{R}^2 \rightarrow \mathbb{R}^3$, where $x$ represents a normalized coordinate grid in $[0, 1]^2$ serving as the input to the INR. Through manipulating the weight vector, we can simulate various image augmentations on the INR's representation. For instance, given a rotation matrix $R \in \mathbb{R}^{2\times2}$, multiplication of the first layer weights $W_1$ with $R$ effectively rotates the image represented by the INR. Following similar principles, we can implement both translation and scaling operations through appropriate weight transformations. For INRs, we apply rotation, translation, and scaling augmentations. Besides all these, we have proposed a more fine-grained augmentation named bias perturbation. Different to directly adding Gaussian noise to both weights and biases, we simple implement the disturbance to the biases. In this way, a more fine-grained augmentation is applied due to different activation value. In addition, for RGB images, we have proposed a series of color jitter augmentations including brightness adjustment, contrast adjustment and saturation adjustment. See \cref{fig:aug} for the example of our proposed data augmentations.

\section{Equivariant Architecture}
To construct our equivariant encoder, we follow the framework established in \cite{equivariant}. The weight space $V$ is decomposed into $\mathcal{V}=\mathcal{W} \oplus \mathcal{B}$, where $\mathcal{W}:=\bigoplus_{m=1}^{M} \mathcal{W}_{m}$ and $\mathcal{B}:=\bigoplus_{m=1}^{M} \mathcal{B}_{m}$ represent the weight and bias spaces, respectively. The equivariant layer $L$ is partitioned into four mappings: $L_{\mathrm{ww}}: \mathcal{W} \rightarrow \mathcal{W}$, $L_{\mathrm{wb}}: \mathcal{W} \rightarrow \mathcal{B}$, $L_{\mathrm{bw}}: \mathcal{B} \rightarrow \mathcal{W}$, and $L_{\mathrm{bb}}: \mathcal{B} \rightarrow \mathcal{B}$. These mappings are implemented using standard equivariant operations (pooling, broadcast, and linear layers) as described in \cite{deepset,deepset2}. Our implementation follows the block matrix structure from \cite{equivariant}, with modifications to the layer configuration and an additional projection layer.

\section{Implementation Details}
Our equivariant architecture is implemented with four hidden equivariant layers followed by a final invariant layer, with the output equivariant feature dimension set to 128. The training process consists of three distinct stages:
First, during the equivariant encoder pre-training stage, we employ the AdamW~\cite{adamw} optimizer with a weight decay of 5e-4 and a learning rate of 5e-3. The encoder is trained for 500 epochs with a batch size of 512.
Second, in the equivariance-guided diffusion stage, we utilize a squared cosine beta scheduler~\cite{improveddiffusion} to modulate noise injection across 1000 timesteps. For MLP sampling from the diffusion process, we implement the Denoising Diffusion Implicit Models (DDIM)~\cite{ddim}. For the transformer architecture, we follow the modified version of minGPT~\cite{Peebles2022} which has 12 layers, 16 self-attention heads and 2880 hidden size. The input MLP is flattened into a 1D vector and projects to 6 tokens (weight and bias from each layer form 2 distinct tokens, our MLP has 3 layers, so that's 6 in total). We also incorporate an Exponential Moving Average (EMA) strategy with $\beta = 0.99$ to enhance convergence stability. This stage comprises 5000 epochs of training using the AdamW optimizer with a batch size of 32 and an initial learning rate of 2e-4, employing a decay schedule that reduces the learning rate by 10\% every 250 epochs. The equivariance loss proportion parameter $\lambda$ is set to 0.1 unless otherwise specified. The process of fine-tuning $\lambda$ is demonstrated in subsequent sections
Finally, during the few-shot fine-tuning stage, we maintain identical configurations to the previous stage while training for 250 epochs. 
At last, the subspace disturbance parameter $\gamma$ in the generation process is set to 0.3 by default. All experiments are conducted on the Linux server with two L20 GPUs.

\section{Additional Experimental Results}

\begin{table}[t]
\centering
\caption{Quantitative evaluation of different shot generation on both MNIST-INRs, CIFAR-10-INRs.}
\label{fig:shots}
% \resizebox{\columnwidth}{!}{%
\begin{tabular}{c|cc|cc}
\toprule
\multirow{2}{*}{Shots} & \multicolumn{2}{|c|}{MNIST-INRs}                               & \multicolumn{2}{c}{CIFAR10-INRs}  \\ \cmidrule(l){2-5} 
 &
  FID$\downarrow$ &
  \multicolumn{1}{c|}{LPIPS$\uparrow$} &
  \multicolumn{1}{c}{FID$\downarrow$} &
  \multicolumn{1}{c}{LPIPS$\uparrow$} \\ \midrule
1-Shot            &       185.80    & \multicolumn{1}{c|}{0.2169}  &\multicolumn{1}{c}{202.70} & \multicolumn{1}{c}{0.2561}            \\
3-Shot            &   143.55            &   0.2907     &  180.72& 0.3319\\
5-Shot             &  \underline{127.39}     &    \underline{0.3355}    &   \underline{165.43}    &  \underline{0.3702}   \\
10-Shot           &  \textbf{121.24}&      \textbf{0.4133}                   &  \textbf{164.14}             & \textbf{0.4926}    \\ \bottomrule
\end{tabular}%
% }
\end{table}

\begin{table}[t]
\caption{Quantitative evaluation of different shot generation on ShapeNet-INRs.}
\label{fig:shot2}
\begin{tabular}{c|c|ccc}
\toprule
\multicolumn{1}{c|}{Category} & \multicolumn{1}{c|}{Shots} & \multicolumn{1}{c}{MMD$\downarrow$} & COV(\%)$\uparrow$ & 1-NNA(\%)$\downarrow$ \\ \midrule
\multicolumn{1}{c|}{\multirow{4}{*}{Airplane}} & \multicolumn{1}{c|}{1-shot} & \multicolumn{1}{c}{4.8} & 20 & 85.2 \\
\multicolumn{1}{c|}{} & \multicolumn{1}{c|}{3-shot} & \multicolumn{1}{c}{4.1} & 26 & 79.5 \\
\multicolumn{1}{c|}{} & 5-shot & \underline{3.7} & \underline{31} & \underline{75.8} \\
\multicolumn{1}{c|}{} & 10-shot & \textbf{3.4} & \textbf{35} & \textbf{73.0} \\ \midrule
\multirow{4}{*}{Car} & 1-shot & 5.0 & 18 & 88.3 \\
 & 3-shot & 4.2 & 23 & 82.4 \\
 & 5-shot & \underline{3.8} & \underline{27} & \underline{79.1} \\
 & 10-shot & \textbf{3.5} & \textbf{31} & \textbf{76.5} \\ \midrule
\multirow{4}{*}{Chair} & 1-shot & 5.8 & 25 & 79.5 \\
 & 3-shot & 4.9 & 32 & 73.2 \\
 & 5-shot & \underline{4.5} & \underline{37} & \underline{69.8} \\
 & 10-shot & \textbf{4.2} & \textbf{41} & \textbf{67.1} \\ \bottomrule
\end{tabular}
\end{table}

\noindent\textbf{Impact of few-shot sample numbers.}
As demonstrated in Tables \ref{fig:shots} and \ref{fig:shot2}, our experimental results validate the consistency of both quality and diversity metrics across varying quantities of few-shot support samples. The inverse relationship between sample size and learning complexity manifests in the evaluation metrics: specifically, the FID for 2D scenarios and MMD for 3D scenarios exhibit elevated values, indicating degraded generation quality with reduced sample sizes. Similarly, for generative diversity metrics, LPIPS for 2D and COV for 3D scenarios demonstrate performance deterioration proportional to the reduction in support samples.

\noindent\textbf{Additional ablation study.}
Similar results to 3D scenario in the main paper are obtained. As illustrated in \cref{fig:ab2d}, we conducted a detailed ablation analysis to evaluate the distinct effects of weight space smooth augmentation and equivariant subspace disturbance in 2D scenarios. The experimental results demonstrate that smooth augmentation independently improves both generation quality and diversity metrics. This finding corroborates that initialized from an optimized state, the equivariant encoder achieves enhanced representational capacity through contrastive learning. In contrast, the application of subspace disturbance alone yields higher diversity scores but exhibits a slight degradation in generation quality when implemented without smooth augmentation. This performance trade-off can be attributed to the divergent categorical clustering of equivariant features under identical disturbance conditions, contingent upon the presence or absence of smooth augmentation. Notably, the concurrent implementation of both components—smooth augmentation and subspace disturbance—yields optimal performance across all metrics.

\noindent\textbf{Additional exploration of equivariant subspace.}
As a complementary to the 2D t-SNE visualization of the equivariant space, we offer the training loss both with and without the smooth augmentation on the MNIST-INRs in Fig \cref{fig:loss}. A comparatively faster converging speed and an obvious better final loss is obtained if the weights have been smooth augmented.

\begin{table}[t]

\caption{Ablation study of weight space smooth augmentation and equivariant space disturbance on MNIST-INRs and CIFAR-10-INRs. Combined usage achieves optimal performance, while individual modules demonstrate distinct contributions to quality and diversity.}
\label{fig:ab2d}
\footnotesize
\centering
\begin{tabular}{c|cc|cc}
\toprule
                     Dataset  & Smooth & \multicolumn{1}{c|}{Disturbance} & \multicolumn{1}{c}{FID$\downarrow$} & \multicolumn{1}{c}{LPIPS$\uparrow$}  \\ \midrule
\multirow{4}{*}{MNIST-INRs} &   \textcolor{purple}{$\usym{2717}$}  & \multicolumn{1}{c|}{\textcolor{purple}{$\usym{2717}$}}  & 137.54    &  0.3357   \\
                         &      \textcolor{teal}{$\usym{2713}$}     & \multicolumn{1}{c|}{\textcolor{purple}{$\usym{2717}$}} & \textbf{120.15} &  0.3466  \\
                         &      \textcolor{purple}{$\usym{2717}$}                &      \textcolor{teal}{$\usym{2713}$}                 &   139.65                   &  \underline{0.3988}  \\
                         &             \textcolor{teal}{$\usym{2713}$}         &       \textcolor{teal}{$\usym{2713}$}                &        \underline{121.24}             & \textbf{0.4133}  \\ \midrule
\multirow{4}{*}{CIFAR10-INRs} & \textcolor{purple}{$\usym{2717}$}        &\textcolor{purple}{$\usym{2717}$}                       &   187.09      &  0.3974  \\
                         & \multicolumn{1}{c}{\textcolor{teal}{$\usym{2713}$}} &          \textcolor{purple}{$\usym{2717}$}             &    \textbf{157.83}         &  0.4175  \\
                         & \multicolumn{1}{c}{\textcolor{purple}{$\usym{2717}$}} &     \textcolor{teal}{$\usym{2713}$}                  & 192.57             &  \textbf{0.4841}  \\
                         & \multicolumn{1}{c}{\textcolor{teal}{$\usym{2713}$}} &          \textcolor{teal}{$\usym{2713}$}             &       \underline{164.14}            & \underline{0.4822}\\ \bottomrule
\end{tabular}%

\end{table}

\begin{figure}[t]
    \centering
    \includegraphics[width=1\linewidth]{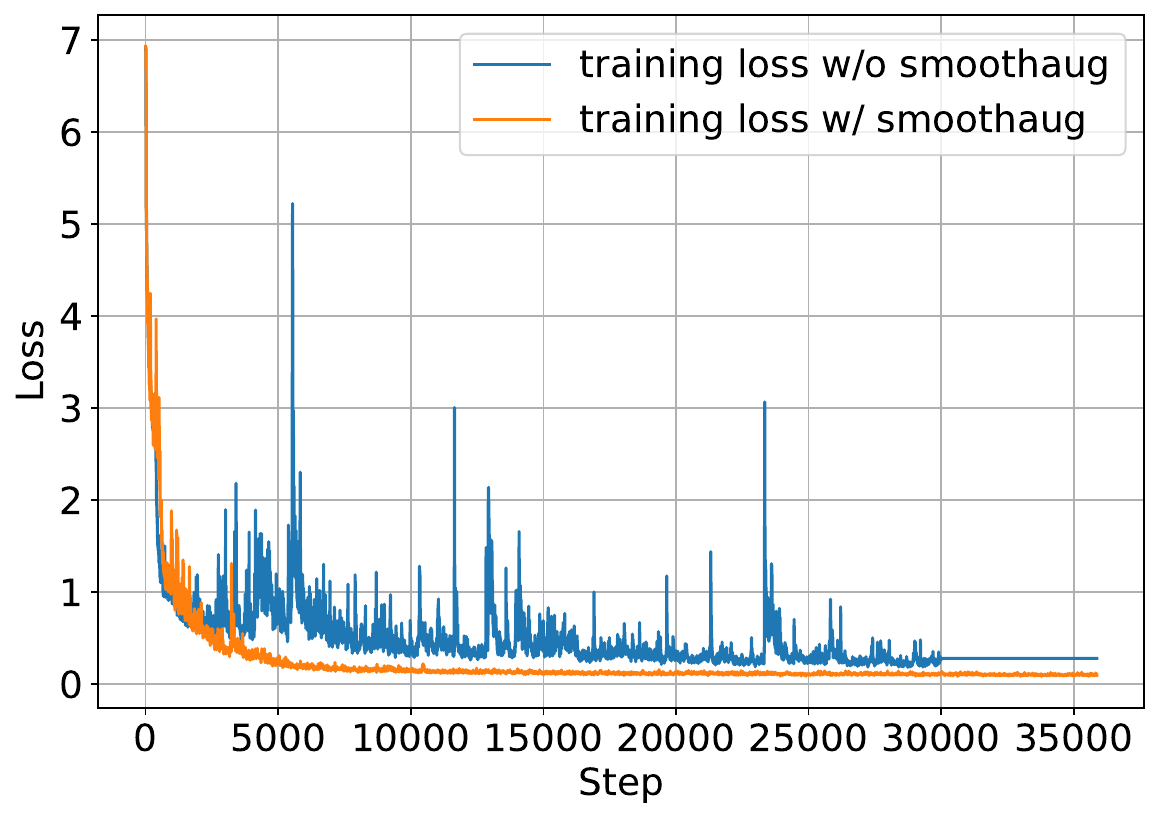}
    \caption{The training loss of the equivariant encoder pre-training. With and without smooth augmentation show notable differences in terms of the converging speed and the final converged loss.}
    \label{fig:loss}
\end{figure}

\begin{figure}[t]
    \centering
    \includegraphics[width=1\linewidth]{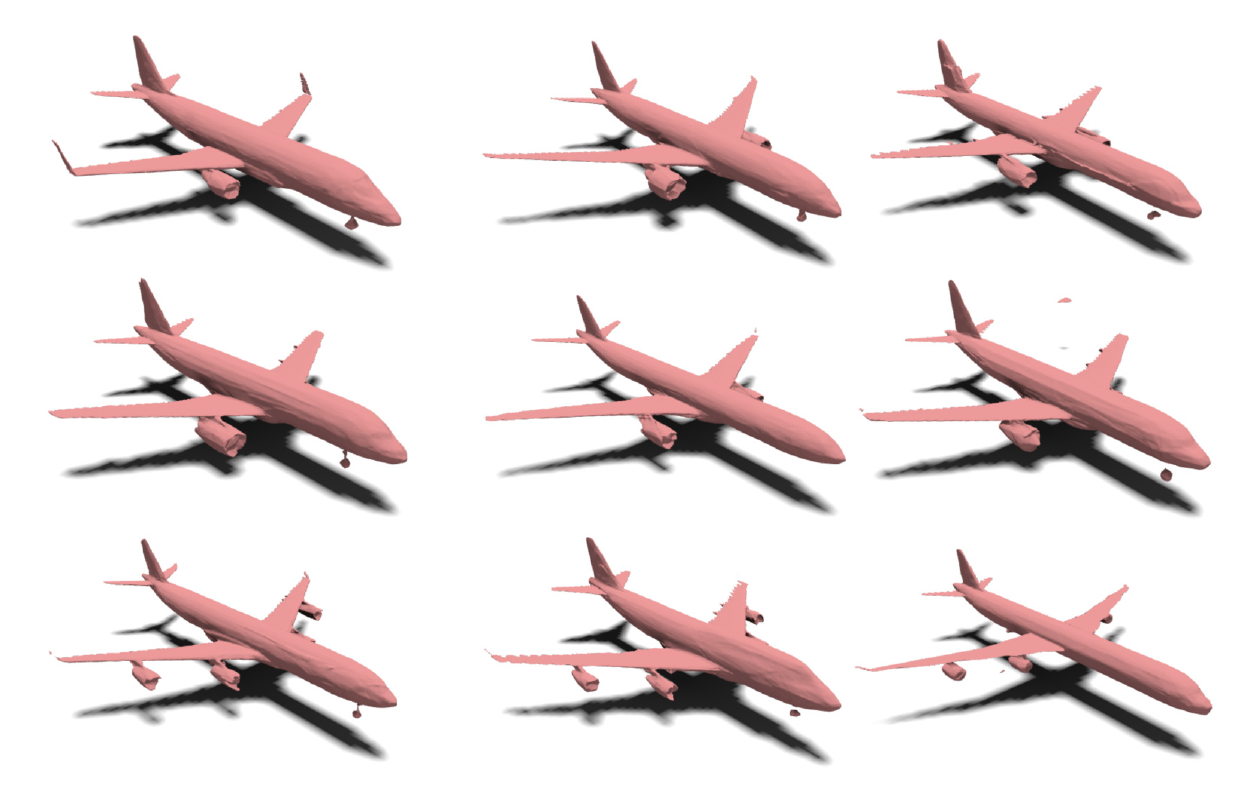}
    \caption{Qualitative comparison of 3-shot generation results on the plane category of ShapeNet-INRs dataset. Notable geometric variations are exhibited across structural components, particularly in the configuration of wings, engine placements, and nose cone morphologies. Left: Support samples. Right: Generated samples.}
    \label{fig:plane}
\end{figure}

\begin{figure}[t]
    \centering
    \includegraphics[width=1\linewidth]{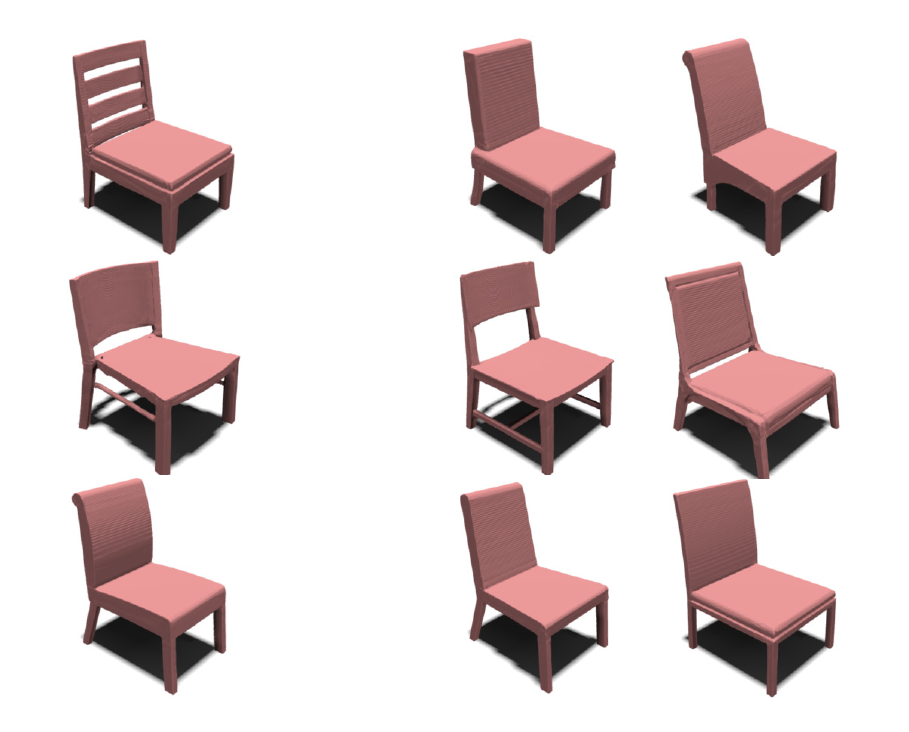}
    \caption{Qualitative comparison of 3-shot generation results on the chair category of ShapeNet-INRs dataset. Notable geometric variations are exhibited across structural components, particularly in the morphology of backrests, leg configurations, and cushion designs. Left: Support samples. Right: Generated samples.}
    \label{fig:chair}
\end{figure}

\begin{figure}[t]
    \centering
    \includegraphics[width=1\linewidth]{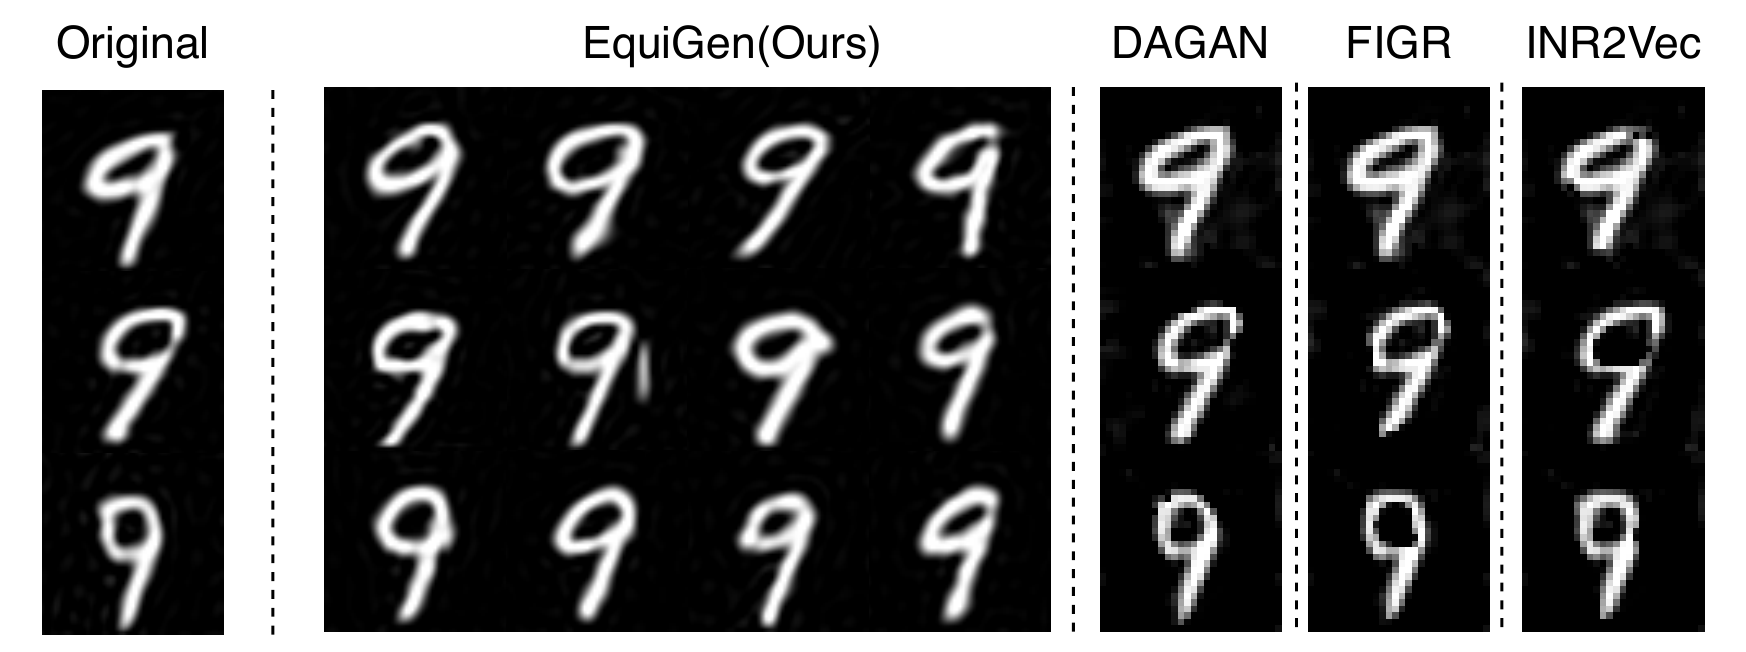}
    \caption{Qualitative results of 3-shot generation on MNIST-INRs. Compared to DAGAN, FIGR and INR2Vec, our method could provide obvious more diverse results.}
    \label{fig:mnistfig}
\end{figure}

\noindent\textbf{Impact of subspace disturbance.}
Similar to 3D scenario in the main paper, through quantitative assessment of equivariant subspace disturbance magnitude and its resultant effects on generative performance, as depicted in \cref{fig:noise_supp}, we identify a significant inverse relationship between sample diversity and functional fidelity. Our analysis reveals that the magnitude of subspace disturbance demonstrates a positive correlation with generation variance. Empirical evidence from \cref{fig:lpips} indicates that elevated disturbance magnitudes correspond to increased LPIPS scores, signifying enhanced inter-sample diversity. However, as evidenced in \cref{fig:fid}, this diversification manifests a concomitant degradation in generation quality, quantified by elevated FID metrics.

\begin{figure}[tbp]
    \centering 
    \subfigbottomskip=2pt
    \subfigcapskip=-5pt %设置子图与子标题之间的距离
    \subfigure[COV with different $\gamma$]{
    \includegraphics[width=0.48\linewidth]{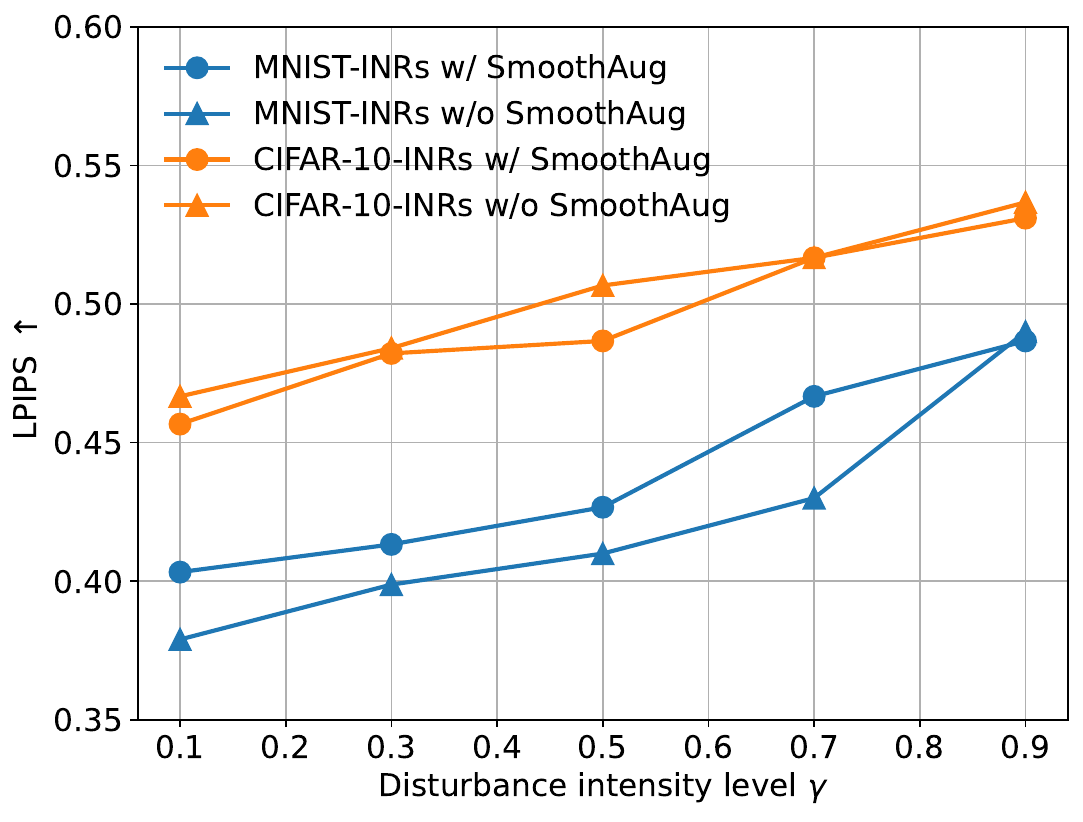}\label{fig:lpips}}
    \subfigure[MMD with different $\gamma$]{
    \includegraphics[width=0.48\linewidth]{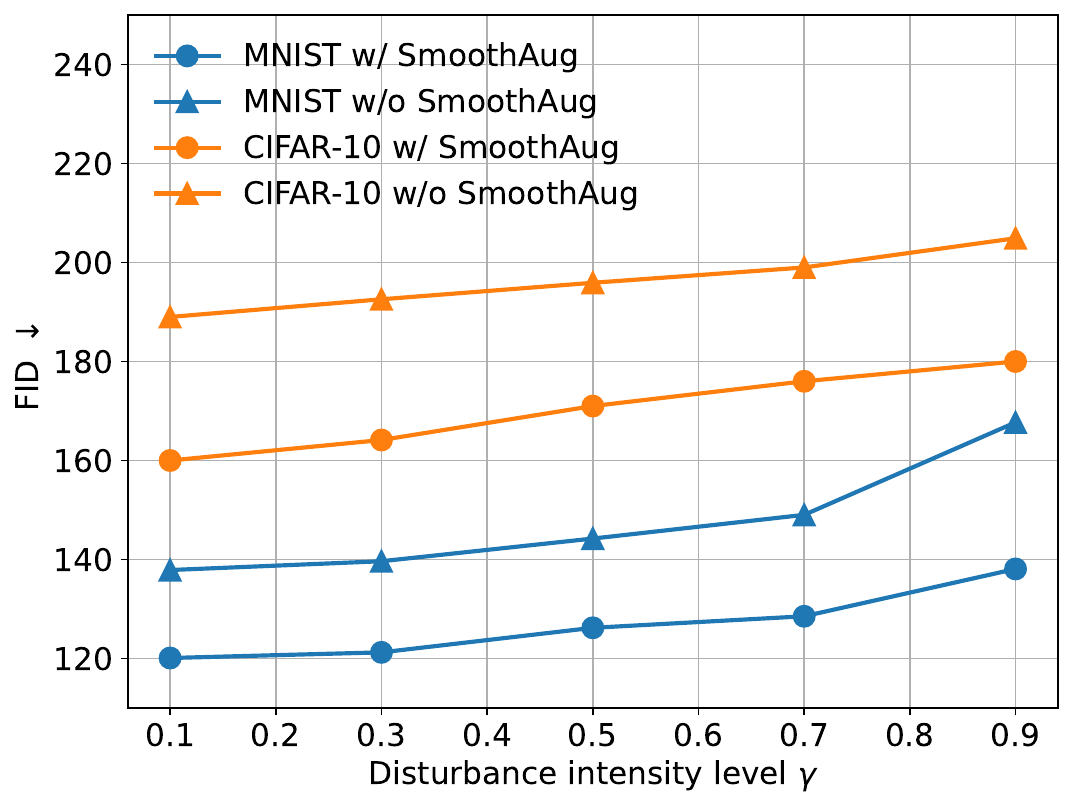}\label{fig:fid}}
    \vspace{-2mm}
    \caption{The evaluation on MNIST-INRs and CIFAR-10-INRs with respect to different subspace disturbance intensity. (a) Higher disturbance leads to increased LPIPS, indicating greater sample diversity. (b) However, larger disturbances result in higher FID, reflecting decreased generation quality.}
    \label{fig:noise_supp}
    \vspace{-6mm}
\end{figure}

\noindent\textbf{Qualitative results.}
To comprehensively evaluate the efficacy of our \algoname, we present additional examples from the ShapeNet-INRs dataset, specifically demonstrating 3-shot generation capabilities across both chair and plane categories. In the context of 3D shape, geometric diversity serves as a critical evaluation criterion. Our analysis reveals obvious structural variations across key components: in the plane category, we observe distinct modifications in wing geometry, engine placement configurations, and nose cone morphologies. Similarly, the chair category exhibits diverse architectural features, manifested through variations in backrest design, leg structure configurations, and cushion geometries.

To intuitively compare the proposed \algoname with existing methods, we visualize the 3-shot generation on MNIST-INRs. As demonstrated in \cref{fig:mnistfig}, our approach generates substantially more diverse outputs compared to baseline methods, which suffer from mode collapse, exhibiting minimal inter-sample variation in their generated results.
To facilitate detailed analysis, we rendered our INR-based results at $56 \times 56$ resolution, leveraging INR's capacity for infinite-resolution rendering. Other baseline methods are rendered at the standard $28 \times 28$ resolution.
